# Supplementary material for: Grounded Intuition of GPT-Vision's Abilities with Scientific Images
Source: arXiv:2311.02069 source file (2023-11-03)
Supplement: Supplementary file 1 [file 2_one-offs.tex]

\section{One-Off Experiments}
\subsection{Typographical Influence}
\label{app:typo_attack}

\subsubsection{Food Labels}
\label{app:food_adversarial}

\subsubsection{Table Caption}
\label{app:table_caption}

\subsection{Lossy Expansion}
\label{app:lossy_exp}
