# Supplementary material for: Grounded Intuition of GPT-Vision's Abilities with Scientific Images
Source: arXiv:2311.02069 source file (2023-11-03)
Supplement: Supplementary file 2 [file 3_longdesc.tex]

\section{Long Descriptions for Alt Text}
stuff
